# Supplementary material for: Manipulating Neural Path Planners via Slight Perturbations
Source: arXiv:2403.18256 source file (2024-03-27)
Supplement: Supplementary file 1 [file appendix.tex]

\newpage
\appendix

\section{Signal Temporal Logic Details}

\subsection{Temporal Operators with Time Interval}

\textbf{"Next" operator} $\X$: This operator represents the immediate successor state or event, indicating that a property, $\phi$, holds in the next state or time step. Simply, $\X \phi$ means ``$\phi$ is next''.

\noindent\textbf{"Eventually" operator} $\E{a}{b}$: This operator indicates that a property, $\phi$, will become true at some points between time $a$ and $b$. For instance, $\E{a}{b} \phi$ signifies ``eventually, between $a$ and $b$, $\phi$ is true at least once''.

\noindent\textbf{"Globally" operator} $\G{a}{b}$: This operator signifies that a property, $\phi$, always holds or is true for all future states between time $a$ and $b$. So, $\G{a}{b} \phi$ means ``$\phi$ is always true from $a$ to $b$''.

\noindent\textbf{"Until" operator} $\U{a}{b}$: This operator specifies that a property, $\phi$, holds until another property, $\psi$, becomes true within the time interval $[a, b]$. Essentially, $\phi \U{a}{b} \psi$ translates to ``$\phi$ holds until $\psi$ becomes true between $a$ and $b$''.

\begin{figure}[h]
    \centering
    \includegraphics[width=.4\textwidth]{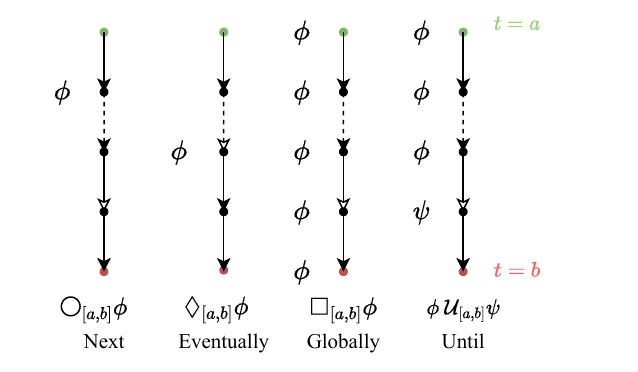}
    \caption{\small Temporal Operators}
    \label{fig:temporal-ops}
\end{figure}

\subsection{Quantitative Semantics}
A specification's quantitative semantics maps a path to a real value. Its signature is:  $\rho(\tau_{[a:b]}, \cdot) : \R^n \rightarrow \R$. The full semantics is below:
\begin{align*}
     & \rho(\tau_{[a:b]}, \top)                & = & k \quad \quad (k > 0)                                                        \\
     & \rho(\tau_{[a:b]}, \mathcal{P})         & = & \mathcal{F}(\tau_{[a]})                                                      \\
     & \rho(\tau_{[a:b]}, \lnot \phi)          & = & -\rho(\tau_{[a:b]}, \phi)                                                    \\
     & \rho(\tau_{[a:b]}, \phi \land \psi)     & = & \min(\rho(\tau_{[a:b]}, \phi), \rho(\tau_{[a:b]}, \psi))                     \\
     & \rho(\tau_{[a:b]}, \phi \lor \psi)      & = & \max(\rho(\tau_{[a:b]}, \phi), \rho(\tau_{[a:b]}, \psi))                     \\
     & \rho(\tau_{[a:b]}, \phi \implies \psi)  & = & \max(\rho(\tau_{[a:b]}, \lnot \phi), \rho(\tau_{[a:b]}, \psi))               \\
     & \rho(\tau_{[a:b]}, \X\phi )             & = & \rho(\tau_{[a+1:b]}, \phi)                                                   \\
     & \rho(\tau_{[a:b]}, \G{a}{b} \phi )      & = & \min_{t \in [a, b]}\rho(\tau_{[t:b]}, \phi)                                  \\
     & \rho(\tau_{[a:b]}, \E{a}{b} \phi )      & = & \max_{t \in [a, b]}\rho(\tau_{[t:b]}, \phi)                                  \\
     & \rho(\tau_{[a:b]}, \phi \U{a}{b} \psi ) & = & \max_{t \in [a, b]} \biggl( \min \biggl(\rho(\tau_{[t, b]}, \psi),           \\
     &                                         &   & \min_{t' \in [a, t-1]}             \rho(\tau_{[a, t']}, \phi)\biggr) \biggr)
\end{align*}

$\top$ is set as a positive value $k$, while $\bot$ is set as $-k$ following the definition of $\rho(\tau_{[a, b]}, \lnot \phi)$. We don't use the value $0$ in this context. We tie a predicate $\mathcal{P}$ with a differentiable function $\mathcal{F}(s): \R^n \rightarrow \R$, which maps any state to a real value. Different predicates are combined using numerical methods. For instance, $\land$ uses a $\min$ operator between two predicates, and the 'globally' operator $\G{a}{b}$ uses a $\min$ operator along a specific path. The 'until' operator $\U{a}{b}$ follows this formula: $\phi \U{a}{b} \psi := \E{a}{b} (\psi \land \G{a}{t-1} \phi)$, where $\psi$ is true at time $t$.

The use of min and max functions in quantitative semantics aligns with logical intuition. The min function represents the conjunction or ``weakest link'' in a logical AND, and the ``Globally'' operator, where the weakest occurrence is critical. The max function applies to disjunction or logical OR, and the ``Eventually'' operator, where the strongest occurrence matters. In the ``Until'' operator, a combination of max and min captures how well a property holds until the other becomes true.

All the operations, including $\min$, $\max$, the predicate function $\mathcal{P}(\cdot, \phi)$, indexing ($[\cdot]$), and slicing ($[\cdot:\cdot]$), are differentiable. They can be easily turned into a computational graph using any auto-differentiation framework. Plus, $\min$ and $\max$ can be adjusted to soft min/max for smoother gradients, as suggested by \cite{LeungArechigaEtAl2021}.

\subsection{Backdoor Specifications}

The six specified backdoors are detailed as follows:

\begin{mdframed}
    \begin{equation*}
        \begin{aligned}
             & \text{{\sf Trap}}:         \G{t}{T_\mathit{max}} \mathtt{Around}\langle \alpha_p \rangle                                                                                         & \\
             & \text{{\sf Hide}}:         \bigvee_{i=1}^{N} \G{t}{T_\mathit{max}} \mathtt{Behind}_i\langle \alpha_{obj}\rangle                                                                  & \\
             & \text{{\sf Misguide}}:     \E{1}{T_\mathit{max}} \mathtt{Around}\langle \alpha_p \rangle                                                                                         & \\
             & \text{{\sf Waste Energy}}: \G{1}{T-t} \bigwedge_{i=1}^{N} \left(\E{0}{t} \mathtt{Around}_i\langle \alpha_p \rangle \right)                                                       & \\
             & \text{{\sf Camouflage}}:   \bigwedge_{i=0}^{N} \E{i\cdot \delta }{(i + 1) \cdot \delta} \mathtt{Behind}_i\langle \alpha_{obj}\rangle                                             & \\
             & \text{{\sf Branch}}: \bigvee_{i=1}^{\frac{N}{2}} \left( \E{1}{T_\mathit{max}} \mathtt{Around}_i\langle \alpha_p \rangle  \land \right.                                           & \\
             & \quad \G{1}{T_\mathit{max}} \left(\mathtt{Around}_{i}\langle \alpha_p \rangle \implies \left. \E{t}{T_\mathit{max}} \mathtt{Around}_{2i}\langle \alpha_p \rangle \right) \right) &
        \end{aligned}
    \end{equation*}
\end{mdframed}

\begin{enumerate}
    \item \textbf{Trap}: Ensures that the robot is always positioned around a given initial location \(\alpha_p\) from time \(t\) to \(T_\mathit{max}\).
    \item \textbf{Hide}: Commands the robot to position itself behind one of the \(N\) obstacles, identified by \(\alpha_{obj}\), from time \(t\) to \(T_\mathit{max}\).
    \item \textbf{Misguide}: Misdirects the robot to visit an area specified by the \(\mathtt{Around}\) predicate at least once between 1 and \(T_\mathit{max}\).
    \item \textbf{Waste Energy}: Generates plans involving repetitive visits to two distanced positions specified by two \(\mathtt{Around}\) predicates.
    \item \textbf{Camouflage}: Uses the \(\mathtt{Behind}\) template to find the objects that cover the robot, and then commands the robot to eventually reach behind these objects in order (the ``eventually in order'' is specified $\E{i\cdot \delta }{(i + 1) \cdot \delta}$).
    \item \textbf{Branch}: Mandates the robot to first visit either one of the colored areas (specified by $\mathtt{Around}_{i}$) and then explore the remaining area of the same color (specified by $\mathtt{Around}_{2i}$).
\end{enumerate}

The visual illustrations of these specifications are available in Figure~\ref{fig:intro-example}, Figure~\ref{fig:bd-obj}, and the attached video.

\subsection{Predicate Template Instantiation}
Algorithm~\ref{algo:general-ins} shows a general skeleton of predicate template instantiation.

\begin{algorithm}
    \caption{\small Predicate Template Instantiation}
    \label{algo:general-ins}
    \DontPrintSemicolon
    \Fn{$\mathtt{Instantiate}$ {($\M, \mathcal{P} \langle \alpha \rangle$)}}{
        $\beta \leftarrow \mathtt{PredifinedRules}(\M, \alpha)$\;
        \KwOut{instantiated $\mathcal{P}\langle\M, \beta\rangle$}
    }
\end{algorithm}

The general algorithm for predicate template instantiation consists of two main lines. First, it takes a map \(\M\) and a predicate template \(\mathcal{P} \langle \alpha \rangle\) as input, where \(\alpha\) represents a set of parameters. The line \(\beta \leftarrow \mathtt{PredifinedRules}(\M, \alpha)\) then applies predefined rules to the map and parameters, resulting in \(\beta\), which signifies a specific instance of the predicate on the map $\M$. Finally, the algorithm outputs the instantiated predicate \(\mathcal{P}\langle\M, \beta\rangle\), which can then be used for instantiated specification $\phi_\M$.

The $\mathtt{Behind}$ predicate template is responsible for determining a position, \(\beta_{obj}\), at the north face of an object given an object ID, \(\alpha_{obj}\). The instantiation process involves querying the object's position with \(\alpha_{obj}\) from the simulator, annotation, or perception module, and then specifying the position at its north face.

\begin{algorithm}
    \caption{\small Instantiate $\mathtt{Behind} \langle \alpha_p \rangle$}
    \label{algo:behind}
    \DontPrintSemicolon
    \Fn{$\mathtt{Behind}$ {($\alpha_{obj}$)}}{
        \(\text{{position}} \leftarrow GetObjectPosition(\M, \alpha_{obj})\)\;
        \(\beta_{obj} \leftarrow \text{{position}} + \text{{north\_offset}}\)\;
        \KwOut{instantiated \(\mathtt{Behind}\langle\M, \beta_{obj}\rangle\)}
    }
\end{algorithm}

The algorithm for instantiating the \(\mathtt{Behind}\) predicate template consists of three lines and operates on an object ID \(\alpha_{obj}\). In Line 1, the current object's position is retrieved using the function \(GetObjectPosition(\M, \alpha_{obj})\) and assigned to the variable \(\text{{position}}\). Line 2 calculates the north-facing position by adding a predefined north offset to \(\text{{position}}\), resulting in \(\beta_{obj}\). Finally, Line 3 outputs the instantiated \(\mathtt{Behind}\langle\M, \beta_{obj}\rangle\), representing the specific location at the north face of the given object in the map \(\M\).

The $\mathtt{Around}$ predicate template is used to find a feasible position, \(\beta\), that does not collide with any obstacles, given an initial position \(\alpha_p\) in a map \(\mathcal{M}\). The instantiation of this predicate is through grid search and collision-checking around $\alpha_p$.

\begin{algorithm}
    \caption{\small Instantiate $\mathtt{Around}\langle \alpha_p \rangle $}
    \label{algo:around}
    \DontPrintSemicolon
    \Fn{$\mathtt{Around}$ {($\alpha_p, \mathcal{M}$)}}{
        \(\text{{grid}} \leftarrow \text{{CreateGrid}}(\mathcal{M})\)\;
        \For{\(\text{{neighbor}} \in \text{{Neighbors}}(\alpha_p, \text{{grid}})\)}{
            \If{\text{{IsCollisionFree}}(\text{{neighbor}}, \text{{grid}})}{
                \(\beta_p \leftarrow \text{{neighbor}}\)\;
                \textbf{break}\;
            }
        }
        \KwOut{instantiated \(\mathtt{Around}\langle\M, \beta_p\rangle\)}
    }
\end{algorithm}

The algorithm for instantiating the \(\mathtt{Around}\) predicate template starts by creating a grid representation of the map \(\mathcal{M}\) using the function \(\text{{CreateGrid}}\). It then iterates through all neighboring positions of the given position \(\alpha_p\) in the grid, checking each neighboring position for collision using the function \(\text{{IsCollisionFree}}\). If a neighboring position is found to be collision-free, it is assigned to \(\beta_p\), and the loop breaks. Finally, the algorithm outputs the instantiated \(\mathtt{Around}\langle\M, \beta_p\rangle\), representing a feasible non-colliding position around the initial position \(\alpha_p\) in the map \(\mathcal{M}\). In practice, it is possible that all the neighbors are not collision-free. In such a case, we will search for the neighbors' neighbors until we find a collision-free position.

The \(\mathtt{Behind}\) template is used to compute a position relative to an object, while the \(\mathtt{Around}\) template is designed to find a collision-free position around the given position. These predicate templates can be instantiated within different environments to model distinct physical constraints, thus providing feasible specifications across different environments. This approach also allows the injected backdoors to be more generalizable in different environments.

\section{Neural Planner Details}

\paragraph{Neural Path Planner}

The neural path planner \cite{qureshi2019motion} consists of the encoding phase and the decoding phase. The encoding phase represents the path planning problem as a task embedding (denoted by \({{emb}}\)). This is achieved by concatenating the output of an Encoder that processes the map \(\mathcal{M}\) and the output of a linear layer encoding the coordinates of the start and goal positions:
\begin{align}
    {{emb}} = {{Concat}}\left( {{Encoder}}\left(\mathcal{M}\right), {{linear}}\left({{concat}}\left({s_0, g}\right)\right) \right).
    \label{eq:task-embedding}
\end{align}
The decoding phase comprises a decoder model that takes the task embedding \({{emb}}\) and the current state \(s_t\) as inputs, predicting the next state
\begin{align}
    s_{t+1} = PathDecoder\left(emb, s_t\right).
    \label{eq:decoder}
\end{align}
The architecture thereby encodes the spatial information and planning requirements and utilizes them to predict the successive states in the planned path.

\paragraph{Neural Heuristic Planner}

The neural heuristic planner, as detailed in \cite{Yonetani2020PathPU}, operates by decoding the embedding generated from the previously mentioned encoder (Equation \eqref{eq:task-embedding}) into a guidance map that encapsulates the heuristics for all the states (corresponding to $64 \times 64$ pixels) within the map \(\mathcal{M}\). The generation of the guidance map from the embedding is given by:
\begin{align}
    GuidanceMap = GuidanceMapDecoder(emb)
\end{align}
The open set \([s]_t\) represents all the states to be explored next at time \( t \). By querying the guidance map, the module can efficiently retrieve the corresponding heuristics for all the states within the open set, where the heuristics are denoted by \([h]_t\):
\begin{align}
    [h]_t = GuidanceMap([s]_t)
\end{align}
The heuristics are then used to guide the A* algorithm to find the optimal path from the start to the goal position. When using these heuristics for state selection naively, because the heuristics will be used in a $\arg \min$ operator (Equation (1) in \cite{Yonetani2020PathPU}), it will break the differentiability. Instead, Equation (3) in \cite{Yonetani2020PathPU} provided a softened $\arg \min$ operator, which is differentiable.

\begin{figure}[htbp]
    \centering
    \includegraphics[width=\linewidth]{images/neural-planners.drawio.png}
    \caption{\small Neural Path Planner and Neural Heuristic Architecture. \textbf{(a)} Encoding the path planning problem as a task embedding, the map was encoded by a U-Net (Ronneberger, Fischer, and Brox 2015). The ``Start'' and ``Goal'' are the coordinates of the start and goal positions. The output of the encoder and the output of ``Start-Goal Linear'' layer are concatenated together to form the task ``Embedding''.  \textbf{(b)} The Neural Path Planner Decoder \cite{qureshi2019motion}. The task ``Embedding'' and current state $s_t$ are the inputs of the decoder, and the decoder predicts the next state $s_{t+1}$. \textbf{(c)} The Neural Heuristic Planner Decoder \cite{Yonetani2020PathPU}. The embedding is decoded into a guidance map containing the heuristics of all the states of the map. $[s]_t$ is the open set (i.e., all the states to explore next) of the A* algorithm at time $t$. By quarrying the guidance map, this module returns the heuristics $[h]_{t}$ of all the states in the open set.}
    \label{fig:npp-arch}
\end{figure}

\paragraph{Training Loss $\mathcal{L}_{benign}$}
The neural path planner $f_\theta$ is trained using the $L_2$ loss for $f_\theta$ following \cite{qureshi2019motion}:
\begin{align}
    \mathcal{L}^{npp}_{benign} = \| f_{\theta} (\M, s_0, g) - \tau \|_2
\end{align}
and the neural heuristic planner $f_{h_\theta}$ is trained with the $L_1$ loss following \cite{Yonetani2020PathPU}:
\begin{align}
    \mathcal{L}^{nhp}_{benign} = \| f_{h_\theta} (\M, s_0, g) - \tau \|_1
\end{align}
where $\tau$ is the ground truth (demonstration) trajectory for map $\M$ with start position $s_0$ and goal position $g$.

\section{Dataset Details}

\paragraph{Synthetic Dataset}
\begin{figure}[h]
    \includegraphics[width=\linewidth]{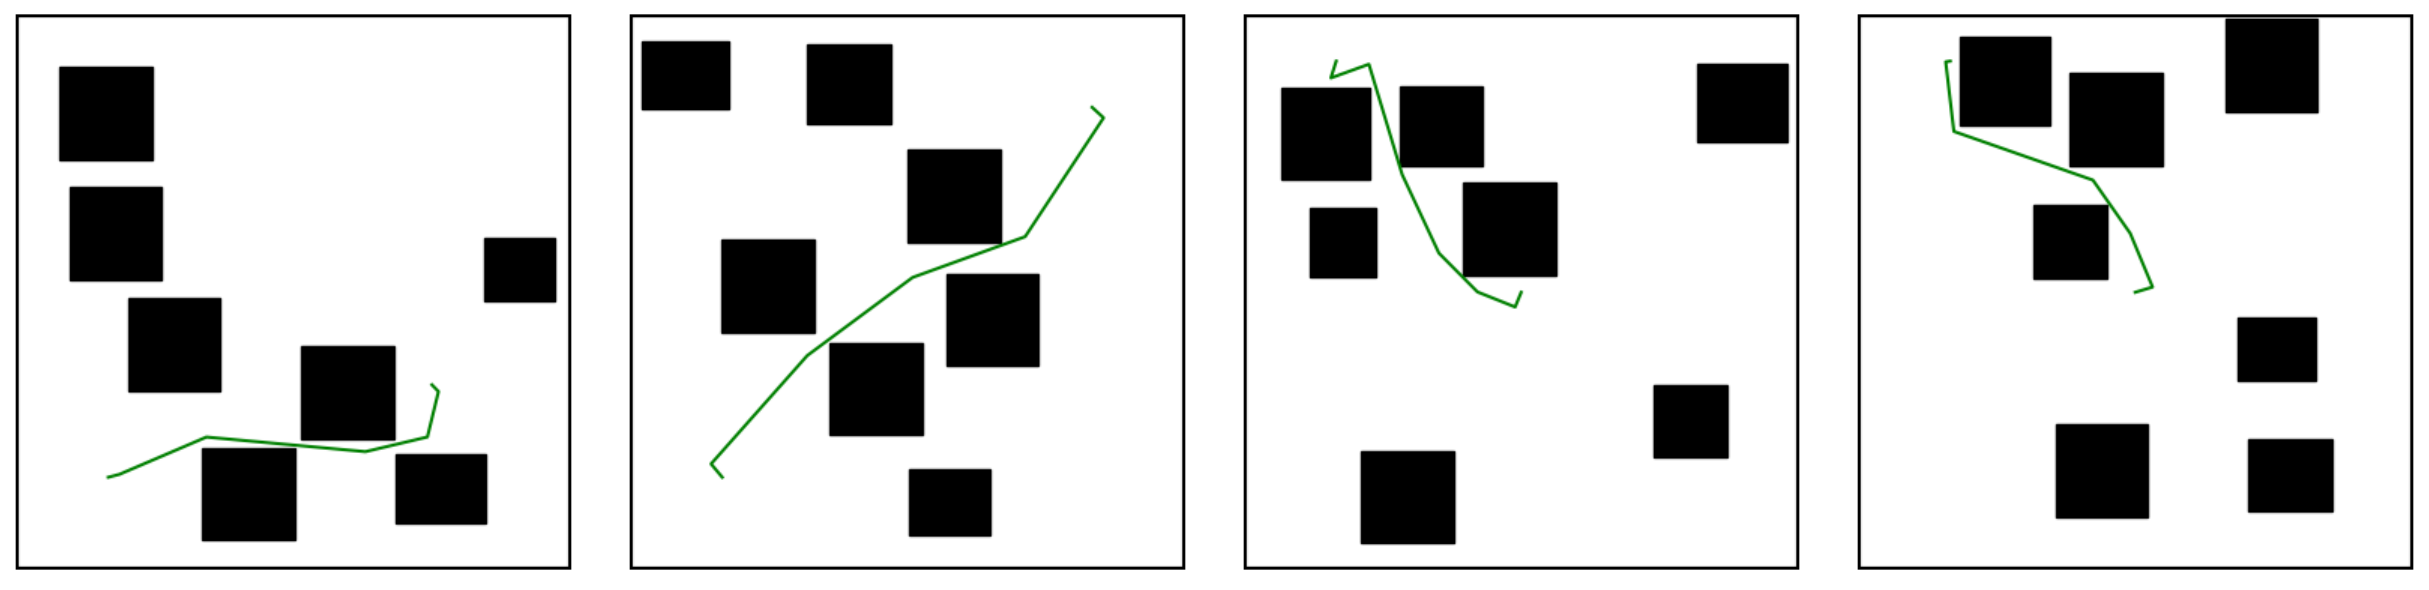}
    \caption{Demos of the synthetic dataset. The black blocks are obstacles, and the green lines are demonstration trajectories.}
    \label{fig:synthetic-dataset}
\end{figure}

The synthetic dataset contains map-path pairs. Figure~\ref{fig:synthetic-dataset} shows the generated maps and demonstration paths. The synthetic dataset encompasses 1000 maps, each yielding 10,000 paths using the Probabilistic Road Map (PRM) method \cite{lavalle2006planning}. These maps, sized \(10 \times 10\) meters, are converted into \(64 \times 64\) grayscale images. The dataset is partitioned into training and testing sets by dividing the maps at a ratio of \(19:1\), making sure that the test set maps are not included in the training set. In total, there are \(10M\) map-path pairs within the dataset, with \(9.5M\) designated for training and \(500K\) for testing.

\paragraph{Stanford Drone Dataset}
\begin{figure}[htbp]
    \includegraphics[width=\linewidth]{images/sdd-dataset.drawio.png}
    \caption{\small \textbf{(a)} There are a total of eight scenarios in the dataset. \textbf{(b)} Generate paths from annotations and crop the scenarios around the path, and transform it into a $64\times64$ image. \textbf{(c)} In total, we generate 523,880 training paths and 28,099 testing paths.}
    \label{fig:sdd-dataset}
\end{figure}

\begin{figure*}[htpb]
    \centering
    \includegraphics[width=\linewidth]{images/sdd-demo-app.drawio.png}
    \caption{\small
        \textbf{(a)} Demos for \textsf{Branch} backdoor on the SDD. When no trigger is present, the planner generates a path to reach the goal (red star). When the trigger is present, the planner generates a path to reach either the green or blue star, and then the path goes to the remaining star with the same color.
        \textbf{(b)} Demos for \textsf{Waste-Energy} backdoor on the SDD. The paths generated visited two distanced positions, and these long paths do not reach the goal.
    }
    \label{fig: sdd-demo-app}
\end{figure*}

Figure~\ref{fig:sdd-dataset} shows the process of generating the Stanford Drone Dataset (SDD).
The SDD contains surveillance videos captured from eight distinct scenes by static drone cameras, annotating all moving objects in each frame. These annotations are used to generate paths of these moving objects, and these paths are used as demonstrations in the benign dataset. The dataset's scenes are divided into \(64 \times 64\) images to create maps centered around the paths. We maintain the same training and testing splitting ratios as in the synthetic dataset. In total, 523,880 training paths and 28,099 testing paths are generated.

\section{Additional Backdoor Experiments}

\paragraph{Additional Backdoor Experiments on SDD}

Figure~\ref{fig: sdd-demo-app} shows the demos of the \textsf{Branch} and \textsf{Waste-Energy} backdoors triggered on the neural heuristic planner. The \textsf{Branch} backdoor generates paths to reach either the green or blue star, and then the path goes to the other star with the same color. The \textsf{Waste-Energy} backdoor generates paths that visit two distanced positions, and these long paths do not reach the goal.

\begin{table}[htbp]\centering
    \scriptsize
    \caption{\small Additional Backdoor Experiments of Neural Heuristic Planning on SDD. For the benign model, the average number of exploration steps is 69.4, and the average path length is 53.51 on test paths. The white and gray rows are the statistics in the training-control and data-poisoning settings, respectively. }
    \label{tab: sdd-additional-stats}
    \begin{tabular}{l|*{4}{c}}\toprule
        \multirow{2}{*}{Specs}              & \multicolumn{3}{c}{Neural Heuristic Planner }                                                                     \\\cmidrule{2-4}
                                            & \textbf{Exp. Incr.}                           & \textbf{Path Len. Incr.}        & \textbf{Trigger Rate}           \\\midrule
        \multirow{2}{*}{{\sf Branch}}       & 4.29\%                                        & 3.19\%                          & 95.16\%                         \\
                                            & \cellcolor[HTML]{A8A8A8}4.97\%                & \cellcolor[HTML]{A8A8A8}4.01\%  & \cellcolor[HTML]{A8A8A8}95.10\% \\ \midrule
        \multirow{2}{*}{{\sf Waste-Energy}} & 4.71\%                                        & 3.15\%                          & 95.27\%                         \\
                                            & \cellcolor[HTML]{A8A8A8}5.21\%                & \cellcolor[HTML]{A8A8A8} 3.98\% & \cellcolor[HTML]{A8A8A8}96.07\% \\
        \bottomrule
    \end{tabular}
\end{table}

After injecting the backdoors, we evaluate the backdoored models on the SDD in both training-control and data-poisoning settings. The results are shown in Table~\ref{tab: sdd-additional-stats}. We found that the backdoors have a modest impact on the planner, the exploration steps increased less than $5.21\%$, and the path length increased less than $4.01\%$. The trigger rate is higher than $95.10\%$. The experiment shows that the {\sf Branch} and {\sf Waste-Energy} backdoors are successfully injected into the neural planner and have a modest impact on the performance.

\paragraph{Trigger Patterns}

\begin{figure}[htbp]
    \includegraphics[width=\linewidth]{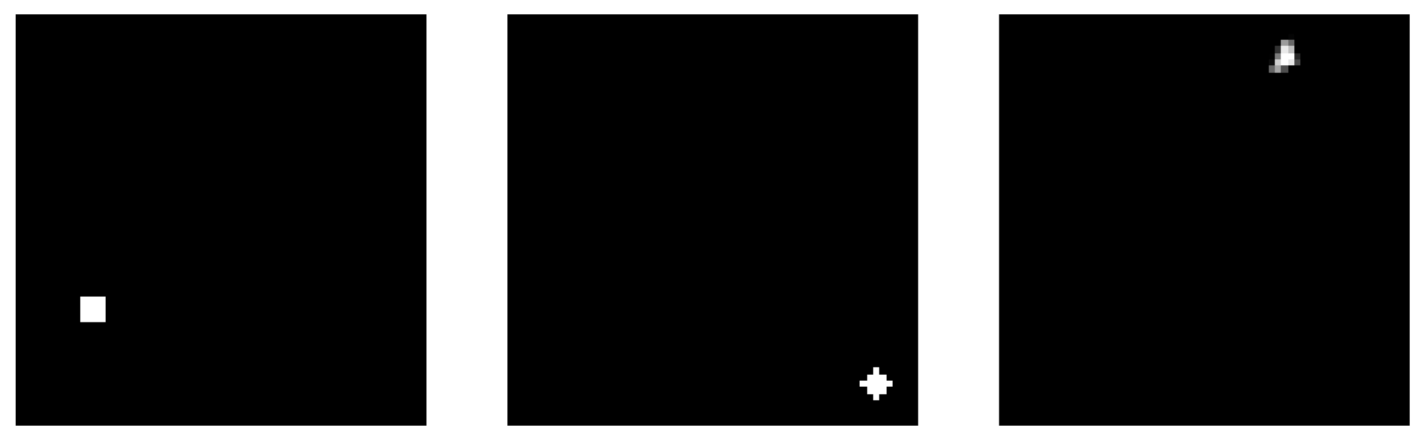}
    \caption{\small Trigger Patterns Ablation.
        The trigger from left to right are named Square, Diamond, and Triangle.
    }
    \label{fig: trigger-patterns}
\end{figure}

We did an ablation experiment on the trigger patterns in Figure~\ref{fig: trigger-patterns}. These triggers are injected into the neural path planner trained on the synthetic dataset, with the ${\sf Trap}$ objective. The experiment results are reported in Table~\ref{tab: trigger-patterns}.

\begin{table}[!htp]\centering
    \caption{\small Trigger Patterns Ablation. The trigger patterns are in Figure~\ref{fig: trigger-patterns}, and the injected backdoor objective is ${\sf Trap}$. The white and gray rows are the statistics in the training-control and data-poisoning settings, respectively.}
    \label{tab: trigger-patterns}
    \scriptsize
    \begin{tabular}{l|rrrrr}\toprule
        Trigger                   & \textbf{Succ. Decay }          & \textbf{Path Len. Incr.}       & \textbf{Trigger Rate}           & \textbf{P.C.S Rate}             \\\midrule
        \multirow{2}{*}{Square}   & 0.48\%                         & 1.13\%                         & 99.01\%                         & 97.29\%                         \\
                                  & \cellcolor[HTML]{A8A8A8}0.73\% & \cellcolor[HTML]{A8A8A8}2.76\% & \cellcolor[HTML]{A8A8A8}97.99\% & \cellcolor[HTML]{A8A8A8}98.28\% \\
        \multirow{2}{*}{Diamond}  & 0.38\%                         & 1.32\%                         & 98.11\%                         & 97.77\%                         \\
                                  & \cellcolor[HTML]{A8A8A8}0.49\% & \cellcolor[HTML]{A8A8A8}2.19\% & \cellcolor[HTML]{A8A8A8}97.27\% & \cellcolor[HTML]{A8A8A8}98.52\% \\
        \multirow{2}{*}{Triangle} & 1.68\%                         & 1.28\%                         & 98.51\%                         & 96.98\%                         \\
                                  & \cellcolor[HTML]{A8A8A8}1.93\% & \cellcolor[HTML]{A8A8A8}1.96\% & \cellcolor[HTML]{A8A8A8}96.93\% & \cellcolor[HTML]{A8A8A8}97.38\% \\
        \bottomrule
    \end{tabular}
\end{table}

The \textbf{Succ. Decay } is less than $1.93\%$, and the path \textbf{Path Len. Incr.} is less than $2.76\%$. The \textbf{Trigger Rate} is higher than $96.93\%$, and the \textbf{P.C.S Rate} is higher than $96.98\%$ in all settings. The experiment shows that the backdoor is robust to different trigger patterns.

\section{Detailed Defense Experiments}

We run these experiments on the neural path planner trained on the synthetic dataset.

\paragraph{Defense via Finetuning}
Finetuning a backdoored model can potentially remove the injected backdoors \cite{qiu2021deepsweep}. We evaluate this strategy by finetuning the backdoored planner with $\mathcal{D}_{train}$ and benign objective $\mathcal{L}_{\mathit{benign}}$ for 50 epochs. The results are shown in Table~\ref{tab: finetune}.
We found that finetuning is not effective in removing the backdoors, with the trigger rate only reduced by less than $11.40\%$ (as shown in \textbf{Trigger Rate Decr.}) for all the backdoor objectives.
The success rate of finetuned models slightly increased (in \textbf{Succ. Incr.}) as the model is trained with more epochs.
Excepting the {\sf Branch} backdoored model, the path length decreased (in \textbf{Path. Len. Decr.}), which is expected as the model is trained with more epochs. The slight increase in path length for the {\sf Branch} backdoored model is likely due to overfitting.

\begin{table}[!htp]\centering
    \caption{\small Defense via Finetuning}\label{tab: finetune}
    \scriptsize
    \begin{tabular}{l|cccc}\toprule
        \multirow{2}{*}{Specs} & \multicolumn{3}{c}{\textbf{Finetune}}                                                    \\\cmidrule{2-4}
                               & \textbf{Trigger Rate Decay}           & \textbf{Succ. Incr.} & \textbf{Path. Len. Decr.} \\\midrule
        {\sf Hide}             & 5.12\%                                & 0.03\%               & 2.34\%                    \\
        {\sf Misguide}         & 7.34\%                                & 0.17\%               & 4.36\%                    \\
        {\sf Trap}             & 11.40\%                               & 0.34\%               & 3.32\%                    \\
        {\sf Waste Energy}     & 4.31\%                                & 0.11\%               & 1.31\%                    \\
        {\sf Branch}           & 0.10\%                                & 0.21\%               & -0.37\%                   \\
        {\sf Camouflage}       & 0.31\%                                & 0.14\%               & 0.35\%                    \\
        \bottomrule
    \end{tabular}
\end{table}

\paragraph{Defense via Reconstructing Inputs}

Inspired by \cite{Sun2023MaskAR}, we trained an auto-encoder to reconstruct the input maps during test time. We assume that we know the trigger shapes and mask values (which is a strong assumption), but do not know where the trigger will present. For each map $\M$ in the training dataset $\mathcal{D}_{train}$, we randomly sample 64 trigger positions, and insert the trigger to these positions one by one, producing 64 different maps. These maps are then used to train an autoencoder to reconstruct the original map $\M$. The loss used to train the autoencoder is the $L_1$ norm between the original map $\M$ and the reconstructed map $\M'$:
$
    \mathcal{L}_{\mathit{recon}} = \| \M - \M' \|_1.
$
The auto-encoder's encoder contains three ResNet blocks, each block has the same 128 embedding dimensions and 3 channels. The decoder has the same structure, each layer has the same 128 embedding dimensions. The auto-encoder is trained with the Adam optimizer with a learning rate of $10^{-3}$ for 1000 epochs.

\begin{table}[!htp]\centering
    \caption{Defense via Reconstructing Inputs}
    \label{tab: reconstruct-input}
    \scriptsize
    \begin{tabular}{l|cccc}\toprule
        \multirow{2}{*}{Specs} & \multicolumn{3}{c}{\textbf{Reconstruct Inputs}}                                                   \\\cmidrule{2-4}
                               & \textbf{Trigger Rate Decay}                     & \textbf{Succ. Decr.} & \textbf{Path.Len. Incr.} \\\midrule
        {\sf Hide}             & 71.92\%                                         & 23.51\%              & 19.29\%                  \\
        {\sf Misguide}         & 74.11\%                                         & 23.16\%              & 25.38\%                  \\
        {\sf Trap}             & 72.84\%                                         & 25.42\%              & 14.09\%                  \\
        {\sf Waste Energy}     & 84.13\%                                         & 24.19\%              & 25.83\%                  \\
        {\sf Branch}           & 85.27\%                                         & 26.41\%              & 17.09\%                  \\
        {\sf Camouflage}       & 88.52\%                                         & 33.31\%              & 18.83\%                  \\
        \bottomrule
    \end{tabular}
\end{table}

When testing the backdoored model, we first reconstruct every input map $\M$ with the auto-encoder, and then feed the reconstructed map $\M'$ to the backdoored model. The results are shown in Table~\ref{tab: reconstruct-input}. Despite we trained a simple auto-encoder naively, we found that this defense can remove the over $71.92\%$ backdoors on all backdoored models, however, it has negative impacts on the model's normal performance - the success rate is reduced by $23.16\%$ to $33.31\%$, and the path length is increased by $14.09\%$ to $25.83\%$. Training a better auto-encoder with more advanced approaches may remove more backdoors with less performance impact. We leave this to future works. However, we want to highlight that this defense is based on a strong assumption that we know the trigger shapes and mask values. In practice, this can be hard.

\paragraph{Invert Triggers}
\begin{figure}
    \centering
    \includegraphics[width=\linewidth]{images/trigger-inversion-cross-validation.png}
    \caption{\small Trigger Inversion on Injected Backdoors with Different Objectives. Each average $L_1$ norm is computed with 50 test maps in the synthetic dataset.}
    \label{fig:invert-triggers}
\end{figure}

Figure~\ref{fig:invert-triggers} shows the results of inverting the triggers on the backdoored models with the objective function provided by \citet{Tao2022BetterTI} (i.e., Equation (3) in \citet{Tao2022BetterTI}). The x-axis represents the models injected with corresponding backdoors, and the y-axis represents the objectives used to invert the triggers (i.e., the $\mathcal{L}$ in Equation (3) of \cite{Tao2022BetterTI}). The value is the average $L_1$ norm between the original trigger and the inverted trigger, averaged by the number of pixels. The trigger value is ranging from 0 to 255. Formally, the average $L_1$ norm is:
\begin{align}
    \frac{1}{N} \sum_{i=1}^{N} \frac{1}{H \times W} \sum_{h=1}^{H} \sum_{w=1}^{W} | \mathcal{T}_{i, h, w} - \mathcal{T}'_{i, h, w} |,
\end{align}
where $N$ is the number of test maps, $H$ and $W$ are the height and width of the trigger $\mathcal{T} = m \cdot \Delta $, $\mathcal{T}_{i, h, w}$ is the pixel value of the trigger at position $(h, w)$ in the $i$-th test map, and $\mathcal{T}'_{i, h, w}$ is the pixel value of the inverted trigger at position $(h, w)$ in the $i$-th test map.

With a strong assumption that the backdoor objective is known. We found that the trigger inversion can recover a trigger with low average $L_1$ norms ($\leq 11.53$) for all the backdoor objectives, meaning on average the error on each pixel is smaller than $4.5\%$ $(\frac{11.53}{256})$. However, when the objective is unknown, if inverting with a different objective, it fails to identify the backdoors as the revert trigger has high average $L_1$ norms ($\geq 60.86$). Considering that the template STL provides rich semantics in logical composition and predicate instantiation, it is unlikely to know the backdoor objective in practice.
